# Supplementary material for: Enhanced sampling of Crystal Nucleation with Graph Representation Learnt Variables
Source: arXiv:2310.07927 ancillary file (2023-10-11)
Supplement: Supplementary file 1 [file SI.pdf]

---

## Supplementary Information

---

Zou and Tiwary

## I. DETAILS ON FEATURIZATION AND MODEL TRAINING

All graphs in this work had their node feature set to be 1 as introduced in the main text. The edge features were expanded under Gaussian basis functions. Here we provided details on featurization and how the model was trained for both systems.

For iron nucleation from the melt, the centers of the  $t$ -th Gaussian are located at  $[0nm, 0.8nm]$  every  $0.05 nm$  with  $\gamma=400 nm^{-2}$ . The GNN model for the iron system consists of one hidden layer of 18 channels in the encoder and zero hidden layers in the decoders. All layers are followed by a ReLU layer except the output layer in the decoders. The model was trained using stochastic gradient descent (SGD) optimizer [1] for 200 epochs. The batch size is 36 and the initial learning rate is 0.01 with 0.1 decreasing every 80 epochs.

For glycine nucleation from the melt, the centers of all angular basis functions are in  $[0, \pi]$  every  $0.1\pi$  step with  $\gamma = 10.13 rad^{-2}$ . The model has zero hidden layers in the encoder which is the same as the decoders to yield efficient computations when performing enhanced sampling without diminishing the ability to classify provided crystalline structures. The model was then trained with SGD optimizer for 65 epochs. The batch size is 256 and the initial learning rate is 0.01 with decrements of 0.5 every 35 epochs.

## II. WELL-TEMPERED METADYNAMICS SIMULATIONS SETUP

285 iron particles were randomly inserted triclinic simulation cell of size  $1.6 \times 1.6 \times 1.6 nm^3$ . The modified embedded-atom (MEAM) interatomic potential introduced by Etesami and Asadi [2] was applied to resemble the optimal physical properties of iron transitions near its melting temperature. All simulations carried out in this work had the equations of motion integrated with a step size of  $2 fs$ . The box was first relaxed with energy minimization, followed by equilibrations in NVT and NPT ensembles separately. The thermostat was selected to be the velocity rescaling thermostat at around experimental melting temperature  $1800 K$  [3] with a coupling time of  $0.1 ps$ . The relaxation time of the barostat [4] was set to be  $10 ps$  and the ambient pressure was set to be the target value. To avoid the formation of unphysical artificial aggregates in atomic simulation [5], changing shape of the simulation cell was enabled.

The simulations of glycine nucleation were performed in a cubic box of size  $2.2 \times 2.2 \times 2.2 nm^3$  with 120 zwitterionic glycine molecules via random insertion. The forcefield parameters are obtained from the general amber forcefield (GAFF) with mB3LYP point charges.[6, 7] The stochastic velocity rescaling thermostat [3] and Parrinello-Rahman barostat [8] were employed with a relaxation time of 0.1 and  $1.0 ps$ , respectively. The reference values were  $500 K$  to the thermostat and  $1.0 bar$  to the barostat. Particle-mesh Ewald method [9] was applied for the computation of long-range electrostatic interaction and hydrogen bonds were constrained with the LINCS algorithm [10]. The cutoffs of electrostatic and Van der Waals interaction in real space were  $0.9 nm$ .

## III. CLASSIFICATION WITH TRAINED LOCAL DECODER IN IRON NUCLEATION

The local decoder predicts the probability of individual nodes in pre-defined class and therefore can be used as an estimator to crystal size. Fig.S1 is the 2-dimensional free energy surface of the size of different crystal packing and the liquid state. The set of subplots suggests it is feasible to form HCP structure from molten iron (subplot (b)) and possible solid-solid transitions may be observed between BCC and HCP iron (subplot (f)).

With a size cutoff of 150, we estimate the free energy differences between the target and initial states as reported in the main text. To examine the reliability of the trained GNN decoder, we benchmark it to the conventional classifying method, adaptive common neighbor analysis. [11] Scatter plots in Fig.S2 suggest the decoder has comparable classification ability in distinguishing crystal structures. Here, we present values of free energy differences computed for comparison in Tab.S1, in addition to a simple local minima approximation method. The results indicate the overall thermodynamic rankings among the three configurations are preserved. The free energy of FCC iron is of large differences which may be due to poor sampling.

## IV. GNN CLASSIFIER FOR GLYCINE POLYMORPHS

As mentioned in the main text, a new GNN model is trained in order to identify all crystalline structures in zwitterionic glycine. Crystallography data including  $\zeta$ -gly [12],  $\epsilon$ -gly [13], and  $\delta$ -gly [13] are used for constructing supercells. Different from previous GNN model (used for biasing), short MD simulations of  $2 ns$  are carried out in

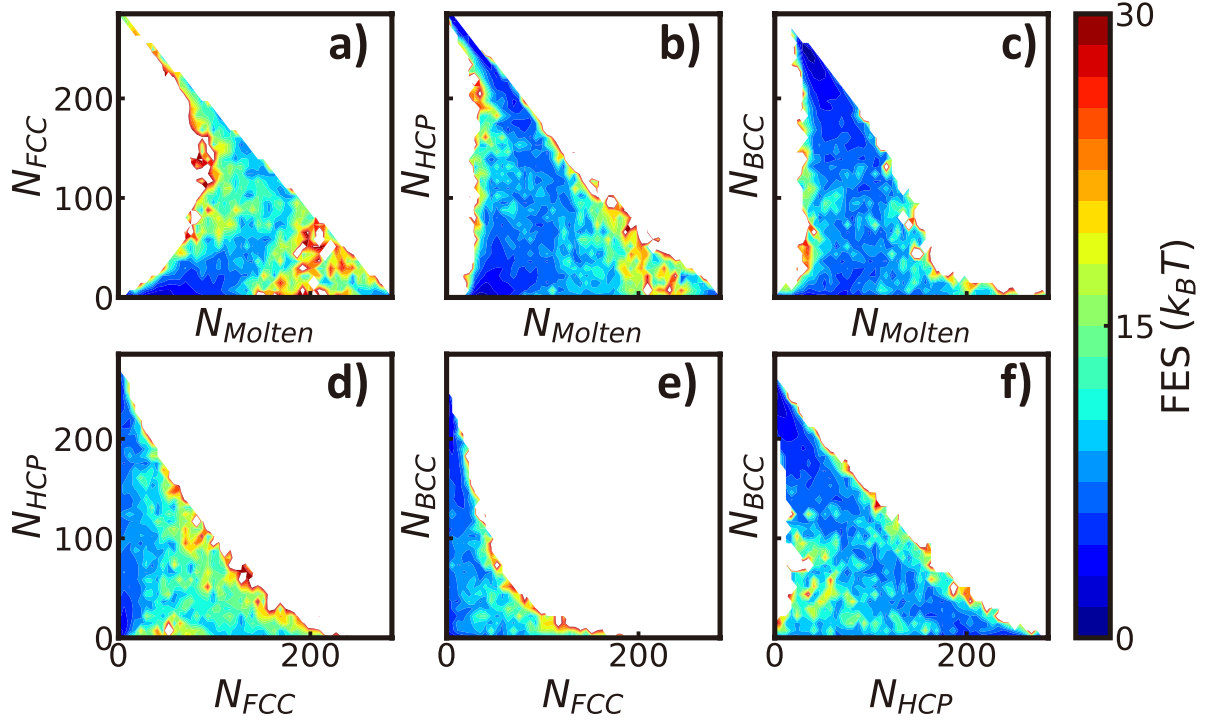

**FIG. S1:** Cluster size of different phases of iron crystals measured by the trained local decoder.

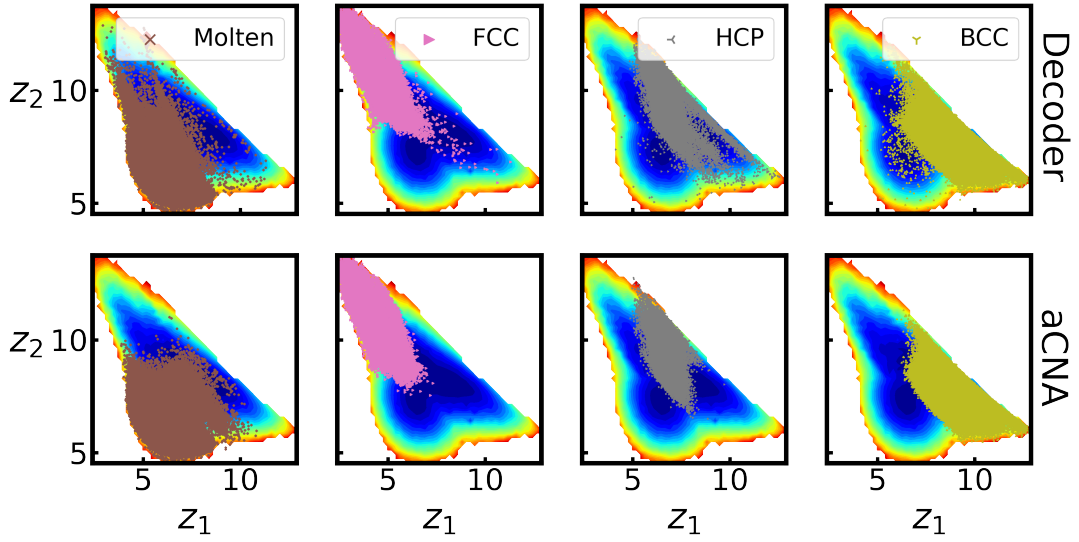

**FIG. S2:** Scatter plots of two classification methods (GNN decoder, upper panel and adaptive common neighbor analysis [11], lower panel) superimpose to reweighted free energy surface from iron nucleation from melts.

TABLE S1: Free energy difference between crystalline phases and molten phase of iron on baseline methods

| System | Transition | Computed free energy difference ( $kJ/mol$ ) |                    |                    |
|--------|------------|----------------------------------------------|--------------------|--------------------|
|        |            | GNN decoder (this work)                      | Local minima       | aCNA               |
| Iron   | M→FCC      | $52.63 \pm 5.63$                             | $188.89 \pm 33.84$ | $148.26 \pm 38.51$ |
|        | M→HCP      | $-20.15 \pm 8.52$                            | $-8.49 \pm 2.61$   | $-15.71 \pm 6.80$  |
|        | M→BCC      | $-34.06 \pm 4.20$                            | $-9.23 \pm 4.73$   | $-33.52 \pm 4.20$  |

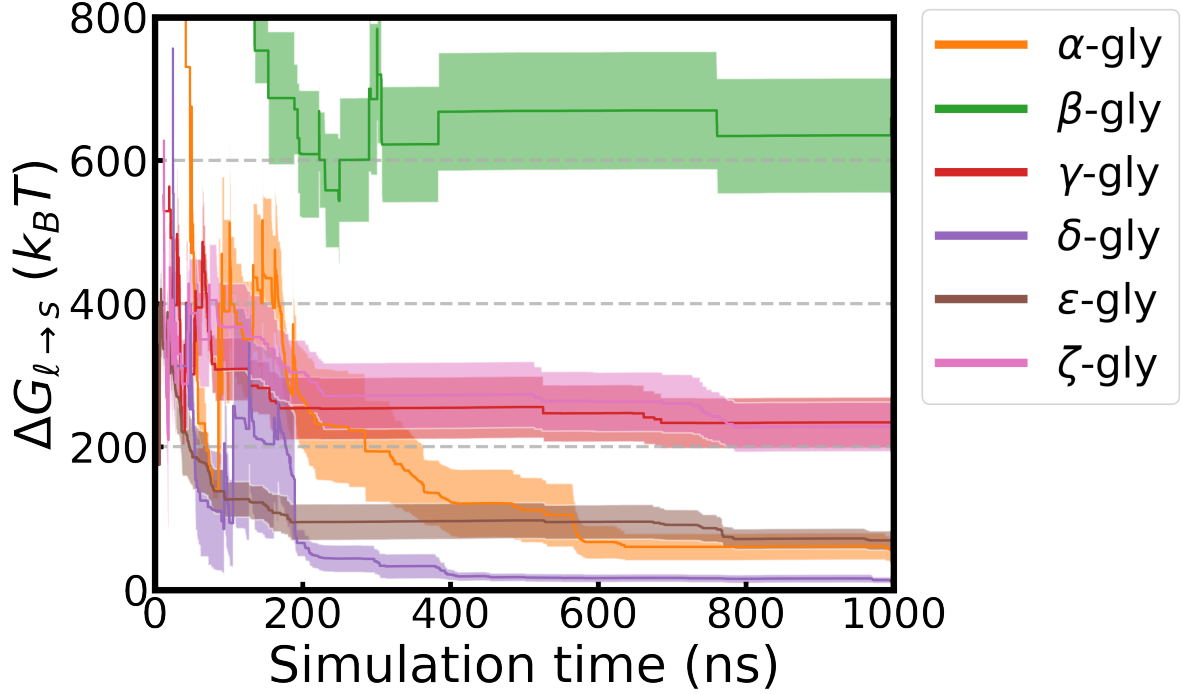

**FIG. S3:**  $\Delta G_{\ell \rightarrow s}$  as a function of simulation time. All high pressure product of glycine are shown to be more stable than glycine polymorphs at ambient condition.

TABLE S2: Free energy difference of crystal structures of glycine polymorphs with respect to the initial molten/liquid phase

| Transition                  | Free energy difference ( $kJ/mol$ ) |
|-----------------------------|-------------------------------------|
| $\ell \rightarrow \alpha$   | $56.43 \pm 16.92$                   |
| $\ell \rightarrow \beta$    | $658.87 \pm 74.72$                  |
| $\ell \rightarrow \gamma$   | $234.11 \pm 35.41$                  |
| $\ell \rightarrow \delta$   | $12.09 \pm 3.41$                    |
| $\ell \rightarrow \epsilon$ | $69.31 \pm 13.44$                   |
| $\ell \rightarrow \zeta$    | $228.12 \pm 34.59$                  |

NVT ensemble to maintain the crystalline structures especially high pressure products without deforming at between 200 to 300  $K$ . 1000 frames of the system are obtained at interval of 0.001  $ps$ .

## V. FREE ENERGY DIFFERENCE TIME SERIES OF GLYCINE POLYMORPHS

Here we plot the free energy difference of all sampled polymorphs of glycine with respect to the liquid phase vs. simulation time in Fig. S3 and the values are reported in Tab. S2. The high pressure polymorphs were identified using the same metric as for the ambient products. The size cutoff was set to be 65 over a total of 120 glycine molecules.

Fig. S4 provides a way of evaluating pathway of underlining solid-solid transitions, where 2-dimensional contour plots were made on the space of size of individual polymorphs identified by the GNN model. Clear evidence of  $\epsilon$ -gly to  $\zeta$ -gly and  $\epsilon$ -gly to  $\gamma$ -gly transitions can be found in Fig. S421) and conversely  $\gamma$ -gly is not likely to form  $\zeta$ -gly directly, this is in agreement to experimental observations as  $\gamma$ -gly to  $\epsilon$ -gly transitions occur at pressures around 4  $GPa$  and  $\epsilon$ -gly transforms into  $\zeta$ -gly as pressure drops to 0.8  $GPa$ . The remaining transitions observed experimentally were not identified in our simulations. [12]

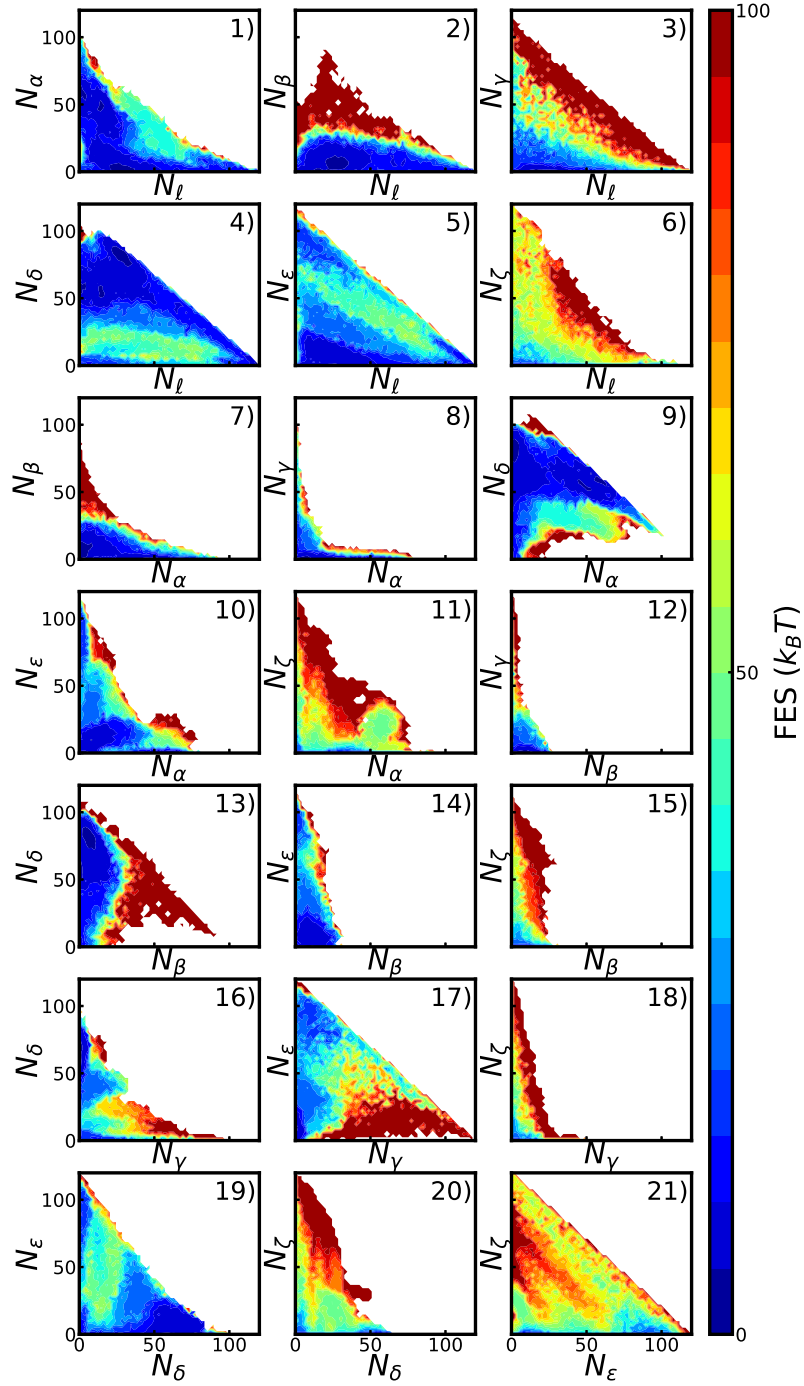

**FIG. S4:** Two-dimensional free energy surfaces of cluster size of different polymorphs of glycine measured by the trained local decoder.

## SUPPLEMENTARY REFERENCES

- 
- [1] S. Ruder, arXiv preprint arXiv:1609.04747 (2016).
  - [2] S. A. Etesami and E. Asadi, Journal of Physics and Chemistry of Solids **112**, 61 (2018).
  - [3] G. Bussi, D. Donadio, and M. Parrinello, J. Chem. Phys. **126**, 014101 (2007).
  - [4] G. J. Martyna, D. J. Tobias, and M. L. Klein, The Journal of chemical physics **101**, 4177 (1994).
  - [5] P. M. Piaggi, O. Valsson, and M. Parrinello, Phys. Rev. Lett. **119**, 015701 (2017).
  - [6] J. Wang, R. M. Wolf, J. W. Caldwell, P. A. Kollman, and D. A. Case, J. Comput. Chem. **25**, 1157 (2004).
  - [7] Y. G. Bushuev, S. V. Davletbaeva, and O. I. Koifman, CrystEngComm **19**, 7197 (2017).
  - [8] M. Parrinello and A. Rahman, Journal of Applied physics **52**, 7182 (1981).
  - [9] U. Essmann, L. Perera, and M. L. Berkowitz, J. Chem. Phys. **103**, 8577 (1995).
  - [10] B. Hess, J. Chem. Theory **4**, 116 (2007).
  - [11] A. Stukowski, Modelling and Simulation in Materials Science and Engineering **20**, 045021 (2012).
  - [12] C. L. Bull, G. Flowitt-Hill, S. de Gironcoli, E. Küçükbenli, S. Parsons, C. H. Pham, H. Y. Playford, and M. G. Tucker, IUCrJ **4**, 569 (2017).
  - [13] A. Dawson, D. R. Allan, S. A. Belmonte, S. J. Clark, W. I. David, P. A. McGregor, S. Parsons, C. R. Pulham, and L. Sawyer, Crystal growth & design **5**, 1415 (2005).
